# Supplementary material for: A Graph Theoretic Approach to Utilizing Protein Structure to Identify Non-Random Somatic Mutations
Source: arXiv:1303.5889 ancillary file (2013-07-12)
Supplement: Supplementary file 1 [file Cosmic_Query.pdf]

Below is the SQL query used to generate the raw data from Cosmic Database version 58.

```
drop table test;
create table test
as
SELECT    GSO.gene_name,SA.id_sample,    upper(REPLACE(sa.sample_name,  '-',''))    as
sample_name,gsm.id_mutation,          SM.AA_mut_start,          SM.AA_MUT_STOP,length(TR.
TRANSCRIPT_AA_SEQ) as AA_len, GSO.swissprot_accession,
SA.ID_SOURCE_SPEC,SA.ID_source,          GSM.ID_MUT_SOMATIC_STATUS,
gsm.ID_MUT_VERIF_STATUS, SA.ID_SOURCE_TISSUE_ORIGIN
FROM    ANALYSED_GENE_SAMPLE  T,  GENE_STUDY  GS,  Gene_sample_mutation  GSM,
sequence_mutation  SM ,cosmic_tumour_sample_overview  SA,  gene_study_transcript  GST,
transcript TR, Gene_SOM GSO
where    GS.id_gene_study    =    T.id_gene_study    and    GSM.id_agc=T.ID_AGS    and
SM.id_mutation=GSM.id_mutation    and    SA.id_sample=T.id_sample    and
GST.id_gene_study=GS.id_gene_study    and    TR.id_transcript    =    GST.ID_TRANSCRIPT    and
GSO.id_gene=TR.id_gene
and GS.WHOLE_GENE_SCREEN='y' and GSM.ID_MUT_SOMATIC_STATUS in (1, 2, 5) and
SM.id_mut_type_AA=22
order by gs.id_gene,SM.AA_mut_start,sa.sample_name;

delete from test
where (id_sample,id_mutation,aa_mut_start) in (select id_sample,id_mutation,aa_mut_start
from test group by id_sample,id_mutation,aa_mut_start having count(*)>1) and rowid not in
(select min(rowid) from test group by id_sample,id_mutation,aa_mut_start having count(*)>1);
select * from test;
```

A visual representation of the table relationships within the database:

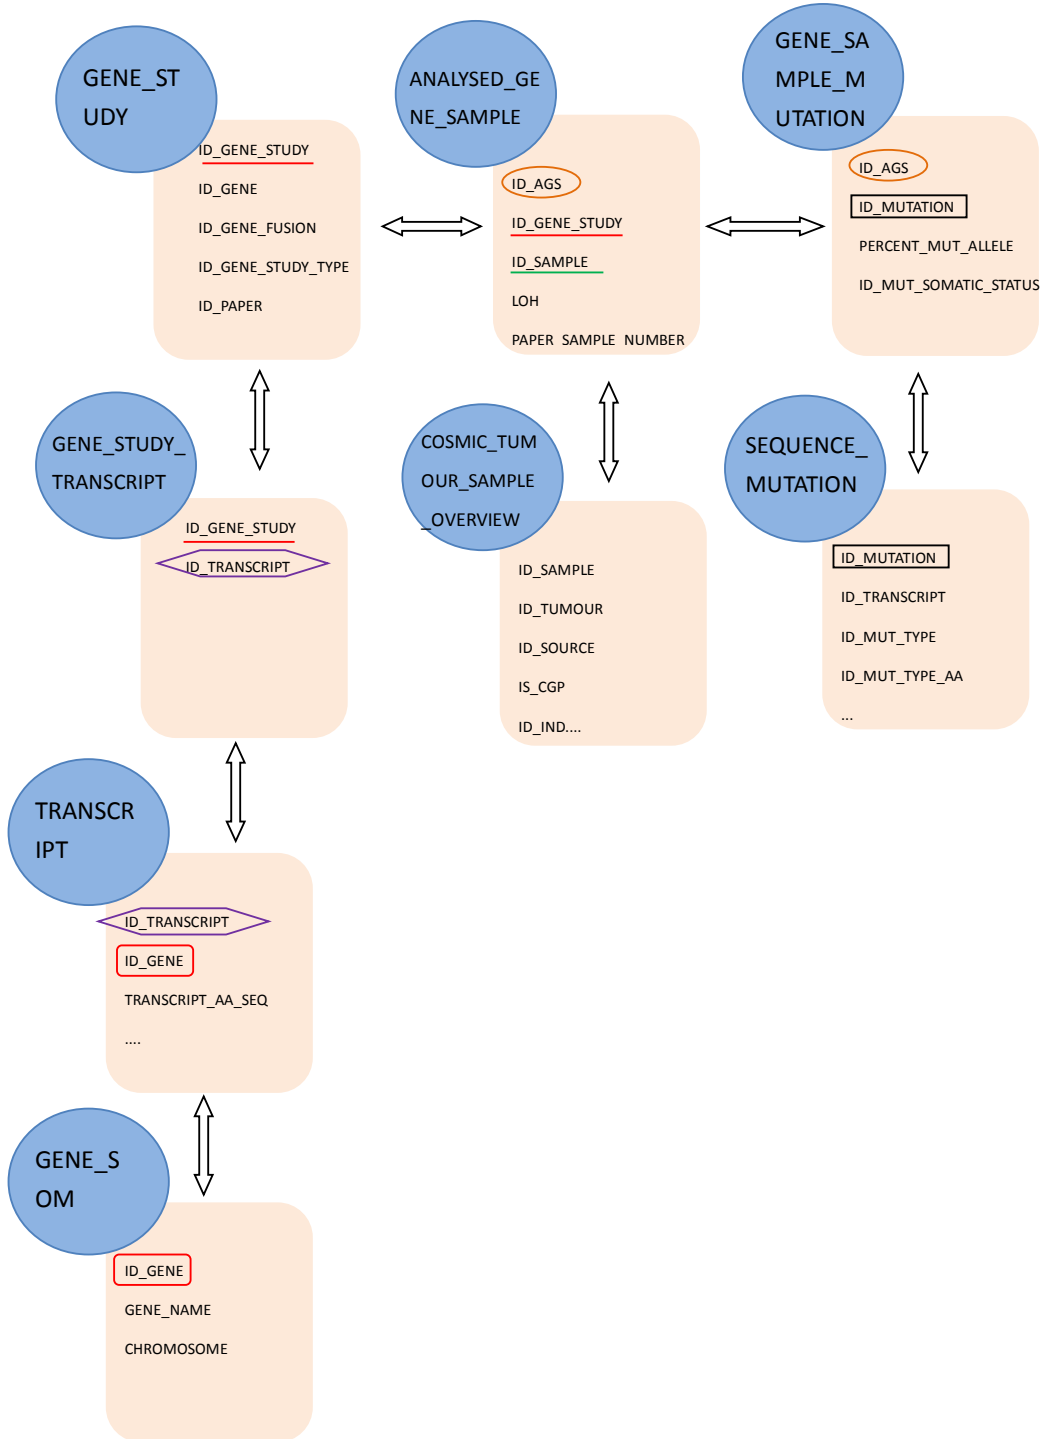

Restrictions imposed upon the mutation accepted for the study.

- 1) COSMIC studies that come to sequencing the whole gene: gene\_study.whole\_gene\_screen = 'y')
- 2) Variants that are somatic: GSM.ID\_MUT\_SOMATIC\_STATUS in (1, 2). Dictionary of mutation status is shown in table 1.

Table 1. Mutation status dictionary in mut\_status\_dic.

|    |                                              |                |
|----|----------------------------------------------|----------------|
| 1  | Confirmed somatic variant                    | somatic_status |
| 2  | Reported in another cancer sample as somatic | somatic_status |
| 3  | Confirmed germline variant                   | somatic_status |
| 21 | Likely cancer causing                        | consequence    |
| 22 | Possible cancer causing                      | consequence    |
| 23 | Unknown consequence                          | consequence    |
| 0  | Not specified                                | somatic_status |
| 4  | Reported in another sample as germline       | somatic_status |
| 5  | Variant of unknown origin                    | somatic_status |
| 6  | Not curated                                  | somatic_status |
| 25 | To be decided                                | consequence    |

3) Mutation type:

Substitution – missense: SM.id\_mut\_type\_AA=22

Table 2. Part of mutation type dictionary in mut\_type\_dic

|    |                              |
|----|------------------------------|
| 11 | Insertion                    |
| 12 | Deletion                     |
| 13 | Complex                      |
| 32 | Nonstop extension            |
| 21 | Substitution - Nonsense      |
| 22 | Substitution - Missense      |
| 23 | Substitution - coding silent |
| 24 | Insertion - In frame         |
| 25 | Insertion - Frameshift       |

- 4) Delete the duplicated rows that have the same gene name, sample number and mutation positions.
